# Supplementary material for: The role of geometric phase in the formation of electronic coherences at conical intersections
Source: arXiv:2011.06728 ancillary file (2020-11-13)
Supplement: Supplementary file 1 [file supplementary.pdf]

# Supplementary information for: The role of geometric phase in the formation of electronic coherences at conical intersections

Simon P. Neville[1], Albert Stolow[1,2,3,4], and Michael S. Schuurman[1,2]

[1] *National Research Council of Canada, 100 Sussex Drive, Ottawa, Ontario K1A 0R6, Canada*

[2] *Department of Chemistry and Biomolecular Sciences, University of Ottawa, 150 Louis Pasteur, Ottawa, Ontario, K1N 6N5, Canada*

[3] *Department of Physics, University of Ottawa, 150 Louis Pasteur,Ottawa, ON K1N 6N5 Canada and*

[4] *University of Ottawa - National Research Council Joint Centre for Extreme Photonics, Ottawa ON K1A 0R6, Canada*

## SYMMETRY PROPERTIES OF TRIGONOMETRIC FUNCTIONS OF THE ADIABATIC-TO-DIABATIC TRANSFORMATION ANGLE

We here discuss in detail the symmetry properties of $\sin 2\theta(q_t, q_c)$ and $\cos 2\theta(q_t, q_c)$ for the case of two electronic states of different symmetry. This discussion is based on a two-mode model, but is valid to all orders of expansion.

In the following we will prove that in the case of a two state, two mode vibronic coupling Hamiltonian, $\sin 2\theta$ and $\cos 2\theta$ are odd and even functions of the coupling mode, respectively, regardless of what order to which the diabatic matrix elements are expanded. We provide two independent proofs. The first is based on an analysis of the Taylor expansion of the diabatic potential matrix about a high-symmetry reference point. The second is centred around a consideration of how the geometric phase (GP) effect manifests itself in the behaviour of the adiabatic-to-diabatic transformation (ADT) angle along a circular contour enclosing a conical intersection (CI).

### Taylor expansion of the diabatic potential matrix

We fix the global gauge of the adiabatic-to-diabatic transformation by taking the adiabatic and diabatic representations to be equal at a point of high (i.e., non-$C_1$) point group symmetry, denoted by $\boldsymbol{Q}_0$. At this geometry, the two adiabatic states $\psi_1^{(a)}$ and $\psi_2^{(a)}$ generate different irreducible representations (irreps) of the point group in question. Thus, the coupling mode $q_c$ generates a non-totally symmetric irrep of the point group, being given by the direct product of the irreps generated by $\psi_1^{(a)}$ and $\psi_2^{(a)}$ at $\boldsymbol{Q}_0$. The tuning mode $q_t$, on the other hand, is totally symmetric by definition.

Let $\boldsymbol{W}(q_t, q_c)$ denote the two-mode, two-state diabatic potential. Being smooth functions of the nuclear coordinates, the elements of $\boldsymbol{W}(q_t, q_c)$ may be expanded in a Taylor series about the reference geometry $\boldsymbol{Q}_0$:

$$W_{ij} = E_i \delta_{ij} + \sum_{\alpha=t,c} \sum_{n=1}^{\infty} \frac{\tau_\alpha^{(i,j;n)}}{n!} q_\alpha^n + \sum_{m=1}^{\infty} \sum_{n=1}^{\infty} \frac{\eta^{(i,j;m,n)}}{(n+m)!} q_t^m q_c^n, \tag{1}$$

where

$$E_i = \left\langle \psi_i^{(a)} \middle| \hat{H}_{el} \middle| \psi_i^{(a)} \right\rangle \Big|_{\boldsymbol{Q}_0} \tag{2}$$

$$\tau_\alpha^{(i,j;n)} = \frac{\partial^n}{\partial q_\alpha^n} \left\langle \psi_i^{(d)} \middle| \hat{H}_{el} \middle| \psi_j^{(d)} \right\rangle \Big|_{\boldsymbol{Q}_0}, \qquad \alpha = t, c, \tag{3}$$

$$\eta^{(i,j;m,n)} = \frac{\partial^{m+n}}{\partial q_t^m \partial q_c^n} \left\langle \psi_i^{(d)} \middle| \hat{H}_{el} \middle| \psi_j^{(d)} \right\rangle \Big|_{\boldsymbol{Q}_0}. \tag{4}$$

By symmetry, only a subset of the coupling coefficients $\tau_\alpha^{(i,j;n)}$ and $\eta^{(i,j;m,n)}$ are non-vanishing. Let $\Gamma^{\text{ts}}$, $\Gamma^t$, $\Gamma^c$, $\Gamma^i$ and denote the totally symmetric irrep, and the irreps generated by $q_t$, $q_c$, $\psi_i^{(a)}(\boldsymbol{Q}_0)$, respectively. Then the following relationships hold:

$$\tau_\alpha^{(i,j;n)} \neq 0 \iff \left[ \bigotimes_{k=1}^{n} \Gamma^\alpha \right] \otimes \Gamma^i \otimes \Gamma^j \subset \Gamma^{\text{ts}}, \tag{5}$$

$$\eta^{(i,j;m,n)} \neq 0 \iff \left[ \bigotimes_{k=1}^{m} \Gamma^t \right] \otimes \left[ \bigotimes_{k=1}^{n} \Gamma^c \right] \otimes \Gamma^i \otimes \Gamma^j \subset \Gamma^{\text{ts}}. \tag{6}$$

Thus, remembering that $\Gamma^t = \Gamma^{\text{ts}}$ and $\Gamma^c = \Gamma^1 \otimes \Gamma^2 \neq \Gamma^{\text{ts}}$, we arrive at the following:

$$\tau_c^{(i,i;n)} \neq 0 \iff n \text{ is even}, \tag{7}$$

$$\tau_c^{(1,2;n)} \neq 0 \iff n \text{ is odd}, \tag{8}$$

$$\eta^{(i,i;m,n)} \neq 0 \iff n \text{ is even}, \tag{9}$$

$$\eta^{(1,2;m,n)} \neq 0 \iff n \text{ is odd}. \tag{10}$$

Using these symmetry relations, we now prove the stated even and odd symmetries of the functions $\cos 2\theta(q_t, q_c)$ and $\sin 2\theta(q_t, q_c)$.

From the relation

$$2\theta(q_t, q_c) = \arctan \Upsilon(q_t, q_c), \tag{11}$$

$$\Upsilon(q_t, q_c) = \frac{2W_{12}(q_t, q_c)}{W_{22}(q_t, q_c) - W_{11}(q_t, q_c)}, \tag{12}$$

we arrive at

$$\cos 2\theta(q_t, q_c) = \sqrt{1 + \Upsilon^2(q_t, q_c)}, \tag{13}$$

and

$$\sin 2\theta(q_t, q_c) = \Upsilon(q_t, q_c)\sqrt{1 + \Upsilon^2(q_t, q_c)}. \tag{14}$$

Using the symmetry relations of Equations 7 to 10, it is clear that $W_{11}$ and $W_{22}$ are both even functions of the coupling mode $q_c$, while $W_{12}$ is an odd function of it. Thus, the function $\Upsilon$ (Equation 12) is an odd function of $q_c$. From Equations 13 and 14, it then follows that the functions $\cos 2\theta(q_t, q_c)$ and $\sin 2\theta(q_t, q_c)$ are even and odd functions of $q_c$, respectively.

**Relation to the geometric phase effect**

As stated in the main text, the symmetry properties of $\cos 2\theta(q_t, q_c)$ and $\sin 2\theta(q_t, q_c)$ with respect to the coupling mode $q_c$ can also be seen to arise from the existence of the GP effect. To see this, consider the evolution of the ADT angle $\theta(q_t, q_c)$ along a circle of radius $r$ centred at the CI point $\boldsymbol{Q}_{CI} = (q_t^{CI}, q_c = 0)$, parameterised as

$$q_t = r\cos\phi + q_t^{CI}, \tag{15}$$

$$q_c = r\sin\phi. \tag{16}$$

Let $\phi_0$ be the polar angle for which $\theta(\phi_0) = 0$ is satisfied. The ADT angle must satisfy $\theta(\phi_0 + \pi) = \pi/2$. This is simply a result of: (i) $q_c$ being equal to zero at this point, and; (ii) the diabatic state energies switching ordering as one completes a half-circuit around the CI. Now, as a result of the GP effect, $\theta(\phi_0 + 2\pi) = \pi$, which gives rise to the double-valued electronic states. We thus see that the ADT angle $\theta(\phi)$ evolves from 0 to $\pi$ as $\phi$ is increased from $\phi_0$ to $\phi_0 + 2\pi$, passing through a value of $\pi/2$ at $\phi = \phi_0 + \pi$. This behaviour (illustrated in Figure 1a) is true for all values of the radius $r$, assuming that the path encircles a single CI. As such, we can conclude that $\cos 2\theta(\phi)$ passes through

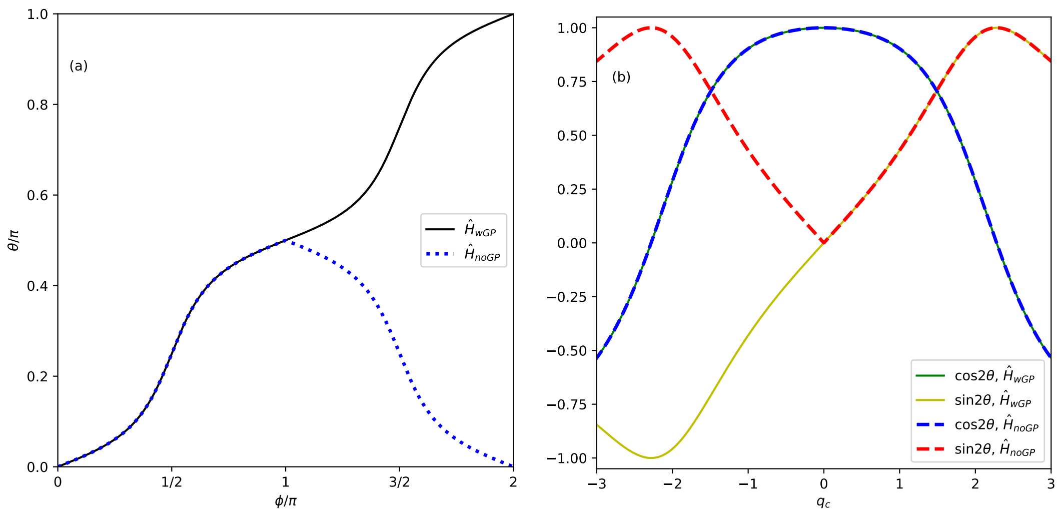


FIG. 1. Symmetries of the ADT angle $\theta(q_t, q_c)$ with and without the geometric phase accounted for (using $\hat{H}_{\mathrm{wGP}}$ and $\hat{H}_{\mathrm{noGP}}$). (a) Evolution of $\theta(q_t, q_c)$ around a unit circle centred at a CI point parameterised as $q_t = r\cos\phi + q_{CI}$, $q_c = r\sin\phi$. (b) $\cos 2\theta(q_t, q_c)$ and $\sin 2\theta(q_t, q_c)$ as a function of the coupling mode $q_c$.

a value of -1 at $\phi = \phi_0 + \pi$, while $\sin 2\theta(\phi)$ passes through zero at this point. Accordingly, $\cos 2\theta(q_t, q_c)$ is found to be an even function of the coupling mode $q_c$, and $\sin 2\theta(q_t, q_c)$ is seen to be an odd function of $q_c$.

For reference, the evolution of the functions $\cos 2\theta$ and $\sin 2\theta$ along a circular path enclosing a CI is shown in Figure 1b. Here, a representative linear vibronic coupling (LVC) Hamiltonian was used, but the observed symmetry properties are general. Shown alongside are the same functions computed using the physically incorrect Hamiltonian $\hat{H}_{\mathrm{noGP}}$ corresponding to the replacement $W_{12} \rightarrow |W_{12}|$ that effectively "turns off" the GP effect. The even and odd symmetries of $\cos 2\theta(q_t, q_c)$ and $\sin 2\theta(q_t, q_c)$ as a function of $q_c$ can clearly be seen in. Furthermore, when the GP effect is not accounted for (here *via* the use of $\hat{H}_{\mathrm{noGP}}$), both $\cos 2\theta(q_t, q_c)$ and $\sin 2\theta(q_t, q_c)$ become artificially even functions of $q_c$.

## SIMILARITY TRANSFORMATION OF THE FIRST-ORDER MODEL OF A CONICAL INTERSECTION

Let $\boldsymbol{W}(x, y)$ denote the two-state diabatic potential expanded around a point of conical intersection (CI), $\boldsymbol{X}_{CI}$, in terms of the intersection-adapted coordinates $(x, y)$. The first-order contribution to $\boldsymbol{W}(x, y)$ reads

$$\boldsymbol{W}^{(1)}(x, y) = (s_x x + s_y y)\,\mathbf{1}_2 + \begin{bmatrix} -gx & hy \\ hy & gx \end{bmatrix}. \tag{17}$$

Here, $g$ and $h$ denote, respectively, the norms of the gradient difference and non-adiabatic coupling vectors, $\boldsymbol{g}$ and $\boldsymbol{h}$, evaluated at the CI point,

$$\boldsymbol{g} \equiv \frac{1}{2}\frac{\partial\,(E_2 - E_1)}{\boldsymbol{X}}\bigg|_{\boldsymbol{X}_{CI}} \tag{18}$$

$$\boldsymbol{h} \equiv \frac{\partial \left\langle \psi_1^{(a)} \middle| \hat{H}_{el} \middle| \psi_2^{(a)} \right\rangle}{\boldsymbol{X}}\Bigg|_{\boldsymbol{X}_{CI}} \tag{19}$$

where $\boldsymbol{X}$ denotes the vector of nuclear coordinates, and $\hat{H}_{el}$ is the electronic Hamiltonian, with eigenvalues $E_j$. The quantities $s_{x/y}$ are the gradients of the average energy with respect to $x$ and $y$ evaluated at $\boldsymbol{X}_{CI}$:

$$s_x \equiv \frac{1}{2}\frac{\partial\left(E_1+E_2\right)}{x}\bigg|_{\boldsymbol{X}_{CI}}, \tag{20}$$

$$s_y \equiv \frac{1}{2}\frac{\partial\left(E_1+E_2\right)}{y}\bigg|_{\boldsymbol{X}_{CI}}. \tag{21}$$

In Equation 17, the adiabatic and diabatic representations are equal at the point of intersection, $\boldsymbol{X_{CI}}$. However, in order to utilise symmetry arguments in the analysis of the propensity to form electronic coherences, it is useful to switch to a diabatic representation in which the adiabatic and diabatic representations are equal at the centre of the initial excited state wavepacket $|\Psi(t=0)\rangle$. We denote this point by $\boldsymbol{X}_0=(x_0,y_0)$.

To proceed, let $\{\psi_j^{(d)}\}$ denote the original set of diabatic states that are equal to the adiabatic states $\{\psi_j^{(a)}\}$ at $\boldsymbol{X}_{CI}$. Let $\boldsymbol{U}(\boldsymbol{X})$ be the corresponding adiabatic-to-diabatic transformation (ADT) matrix,

$$\psi_j^{(d)}(\boldsymbol{X}) = \sum_k U_{kj}(\boldsymbol{X})\psi_k^{(a)}(\boldsymbol{X}). \tag{22}$$

By definition, the ADT matrix $\boldsymbol{U}(\boldsymbol{X})$ satisfies the equation

$$\boldsymbol{F}(\boldsymbol{X})\boldsymbol{U}(\boldsymbol{X}) + \boldsymbol{\nabla}\boldsymbol{U}(\boldsymbol{X}) = 0, \tag{23}$$

where $\boldsymbol{\nabla}$ is the derivative operator with respect to the nuclear coordinates, and$\boldsymbol{F}$ is the matrix of derivative couplings in the adiabatic representation:

$$\boldsymbol{F}_{jk} = \left\langle \psi_j^{(a)} \middle| \boldsymbol{\nabla}\psi_k^{(a)} \right\rangle. \tag{24}$$

Equation 23 only defines the diabatic states up to a constant, nuclear coordinate-independent transformation. That is, given the ADT matrix $\boldsymbol{U}(\boldsymbol{X})$, we may define an entirely equivalent set of diabatic states $\{\tilde{\psi}_j^{(d)}\}$ using a different ADT matrix

$$\tilde{\boldsymbol{U}}(\boldsymbol{X}) = \boldsymbol{U}(\boldsymbol{X})\boldsymbol{T}, \tag{25}$$

where $\boldsymbol{T}$ is a unitary and nuclear coordinate-independent, but otherwise arbitrary, matrix.

We now restrict ourselves to a consideration of dynamics within the branching space. Let $(x_0,y_0)$ be the centre of the initial wavepacket projected onto the branching space. Choosing $\boldsymbol{T}=\boldsymbol{U}^\dagger(x_0,y_0)$, gives

$$\tilde{\boldsymbol{U}}(x_0,y_0) = \boldsymbol{U}(x_0,y_0)\boldsymbol{U}^\dagger(x_0,y_0) = \boldsymbol{1}, \tag{26}$$

which yields diabatic and adiabatic states that are equal at the centre of the initial wavepacket, $(x_0,y_0)$.

The first-order potential potential, $\tilde{\boldsymbol{W}}^{(1)}$, in terms of the new set of diabatic states $\{\tilde{\psi}_j^{(d)}\}$ is obtained from the similarity transformation

$$\tilde{\boldsymbol{W}}^{(1)}(x,y) = \boldsymbol{U}(x_0,y_0)\boldsymbol{W}^{(1)}(x,y)\boldsymbol{U}^\dagger(x_0,y_0). \tag{27}$$

Writing the 'original' ADT matrix $\boldsymbol{U}(x,y)$ as

$$\boldsymbol{U}(x,y) = \begin{bmatrix} \cos\theta(x,y) & \sin\theta(x,y) \\ -\sin\theta(x,y) & \cos\theta(x,y) \end{bmatrix}, \tag{28}$$

we obtain the following expression for the first-order potential in the 'new' diabatic representation:

$$\tilde{\boldsymbol{W}}^{(1)}(x,y) = \left(s_x x + s_y y\right)\boldsymbol{1}_2 + \begin{bmatrix} -\cos\left(2\theta_0\right)gx + \sin\left(2\theta_0\right)hy & \cos\left(2\theta_0\right)hy + \sin\left(2\theta_0\right)gx \\ \cos\left(2\theta_0\right)hy + \sin\left(2\theta_0\right)gx & \cos\left(2\theta_0\right)gx - \sin\left(2\theta_0\right)hy \end{bmatrix}. \tag{29}$$

TABLE I. Values of the tilt parameter $s_y$ used in the LVC Hamiltonians. All values are given in units of eV. $\alpha_y$ denotes the tilt of the cone axis along the non-adiabatic coupling direction.

| $\alpha_y$ | $s_y$ |
|---|---|
| 0.5° | 0.0175 |
| 3° | 0.1054 |
| 7° | 0.2477 |
| 10° | 0.3567 |

TABLE II. Common parameter values used in the LVC Hamiltonians. All values are given in units of eV.

| | |
|---|---|
| $\omega_x$ | 0.10 |
| $\omega_y$ | 0.05 |
| $\Delta$ | 1.00 |
| $\kappa$ | -0.40 |
| $\lambda$ | 0.05 |

## LINEAR VIBRONIC COUPLING HAMILTONIANS USED IN THE CONICAL INTERSECTION TILT ANGLE CALCULATIONS

In the study of the effects of the CI cone axis tilt angle, two-mode linear vibronic coupling (LVC) model Hamiltonians, $\hat{H}_{LVC}$, were constructed to describe ultrafast internal conversion through a CI. In these calculations, dimensionless mass- and frequency-scaled coordinates $q_x$ and $q_y$ were used, and the LVC Hamiltonian matrices took the form

$$\boldsymbol{H}_{LVC} = \frac{1}{2} \sum_{\alpha=x,y} \omega_\alpha \left( q_\alpha^2 - \frac{\partial^2}{\partial q_\alpha^2} \right) \mathbf{1}_2 + s_y q_y \mathbf{1}_2 + \begin{bmatrix} 0 & \lambda q_y \\ \lambda q_y & \Delta + \kappa q_x \end{bmatrix}. \tag{30}$$

Here, the modes $q_x$ and $q_y$ represent the gradient difference and non-adiabatic coupling directions, respectively. The parameter $s_y$ was used to adjust the tilt of the cone axis along the non-adiabatic coupling direction. The different values of the tilt parameter $s_y$ used are given in Table I. The remaining parameters were held at constant values, and these are given in Table II.

The LVC Hamiltonians $\hat{H}_{LVC}$ were used in numerically exact wavepacket propagations in the diabatic representation. The initial state $|\Psi(q_x, q_y, t = 0)\rangle$ was taken as to correspond to vertical excitation of the ground vibronic state to the upper diabatic state $\psi_2^{(d)}$. That is,

$$|\Psi(q_x, q_y, t = 0)\rangle = \left| \psi_2^{(d)} \right\rangle \chi_0(q_x, q_y), \tag{31}$$

where $\chi_0(q_x, q_y)$ is the lowest-lying eigenstate of the zeroth-order Hamiltonian

$$\hat{H}_0 = \frac{1}{2} \sum_{\alpha=x,y} \omega_\alpha \left( q_\alpha^2 - \frac{\partial^2}{\partial q_\alpha^2} \right) \tag{32}$$

The numerically exact representation of the vibronic wavepacket $|\Psi(q_x, q_y, t)\rangle$ used reads

$$|\Psi(q_x, q_y, t)\rangle = \sum_{i=1}^{2} \left| \psi_j^{(d)} \right\rangle \chi_j^{(d)}(q_x, q_y, t), \tag{33}$$

$$\chi_j^{(d)} = \sum_{i_x=1}^{N_x} \sum_{i_y=1}^{N_y} C_{i_x i_y}^{(j)}(t) \zeta_{i_x}^{(x)}(q_x) \zeta_{i_y}^{(y)}(q_y), \tag{34}$$

TABLE III. Numbers $n_\kappa^i$ of SPFs and $N_\kappa$ of primitive harmonic oscillator DVR basis functions used for each mode in the pyrazine MCTDH calculations.

| Mode | $n_\kappa^1, n_\kappa^2$ | $N_\kappa$ |
|---|---|---|
| $\nu_{10a}$ | 7,7 | 22 |
| $\nu_{6a}$ | 12,11 | 32 |
| $\nu_1$ | 6,5 | 21 |
| $\nu_{9a}$ | 5,4 | 12 |

where the primitive basis functions $\zeta_{i_\alpha}^{(\alpha)}(q_\alpha)$ were taken as a harmonic oscillator discrete variable representation (DVR)[1, 2]. In all calculations, the numbers of primitive basis functions used were $N_x = N_y = 105$. The time-dependent Schrödinger equation was solved using the short iterative Lanczos method[3] as implemented in the Quantics quantum dynamics package[4].

## PYRAZINE QUANTUM DYNAMICS CALCULATIONS

For the four-mode, two-state pyrazine model calculations, the wavepacket propagations were performed using the multi-configurational time-dependent Hartree (MCTDH) method[1]. The parameters of the model Hamiltonian were taken from Reference 5 and correspond to an LVC model. The normal modes included in the model are the three totally symmetric tuning modes $\nu_{6a}$, $\nu_1$ and $\nu_{9a}$, and the single coupling mode $\nu_{10a}$, where we have adopted the commonly used normal mode nomenclature of Innes *et al.*[6].

The multi-set formalism without mode combination was used, in which the MCTDH wavefunction *ansatz* for $f$ nuclear degrees of freedom $q_f$ reads

$$|\Psi(q_1,\ldots,q_f,t)\rangle = \sum_{i=1} \left|\Psi^{(i)}(q_1,\ldots,q_f,t)\right\rangle \left|\psi_i^{(d)}\right\rangle, \tag{35}$$

$$\left|\Psi^{(i)}(q_1,\ldots,q_f,t)\right\rangle = \sum_{j_1^i=1}^{n_1^i} \cdots \sum_{j_f^i=1}^{n_f^i} A^{(i)}_{j_1^i,\ldots,j_f^i}(t) \prod_{\kappa=1}^{f} \varphi^{(\kappa,i)}_{j_\kappa^i}(q_\kappa,t). \tag{36}$$

The time-dependent single-particle functions (SPFs) $\varphi_j^{(\kappa,i)}$ are further expanded in terms of a time-independent DVR. Equations of motion for both the expansion coefficients $A^{(I)}_{j_1^I,\ldots,j_p^I}$ and the SPFs are derived variationally, yielding an optimal description of the evolving wavepacket[1]. For all normal modes, a harmonic oscillator DVR was used. The numbers of SPF and DVR functions used for each degree of freedom are given in Table III.


[1] M. H. Beck, A. Jäckle, G. A. Worth, and H. D. Meyer, Physics Reports **324**, 1 (2000).
[2] J. C. Light, I. P. Hamilton, and J. V. Lill, J. Chem. Phys. **82**, 1400 (1985).
[3] T. J. Park and J. C. Light, J. Chem. Phys. **85**, 5870 (1986).
[4] G. A. Worth, K. Giri, G. Richings, I. Burghardt, M. H. Beck, A. Jäckle, and H. D. Meyer, "The quantics package, version 1.1," University of Birmingham, Birmingham, UK (2015).
[5] S. Krempl, M. Winterstetter, H. Plöhn, and W. Domcke, The Journal of Chemical Physics **100**, 926 (1994), https://doi.org/10.1063/1.467253.
[6] K. K. Innes, I. G. Ross, and W. R. Moomaw, J. Mol. Spectrosc. **132**, 492 (1988).
